# Supplementary material for: Non-universal Transverse Electron Mean Free Path through Few-layer Graphene
Source: arXiv:1904.13152 source file (2019-08-21)
Supplement: Supplementary file 1 [file Supplementary_material_mfp_4d.pdf]

# Non-universal Transverse Electron Mean Free Path through Few-layer Graphene

## Supplementary material

D. Geelen,<sup>1</sup> J. Jobst,<sup>1</sup> E.E. Krasovskii,<sup>2,3,4</sup> S.J. van der Molen,<sup>1</sup> and R.M. Tromp<sup>5,1</sup>

<sup>1</sup>Huygens-Kamerlingh Onnes Laboratorium, Leiden Institute of Physics, Leiden University,  
Niels Bohrweg 2, P.O. Box 9504, NL-2300 RA Leiden, The Netherlands

<sup>2</sup>Departamento de Física de Materiales, Universidad del País Vasco UPV/EHU, 20080 San Sebastian/Donostia, Spain

<sup>3</sup>IKERBASQUE, Basque Foundation for Science, E-48013 Bilbao, Spain

<sup>4</sup>Donostia International Physics Center (DIPC), E-20018 San Sebastián, Spain

<sup>5</sup>IBM T.J. Watson Research Center, 1101 Kitchawan Road,

P.O. Box 218, Yorktown Heights, New York, New York 10598, USA

rtromp@us.ibm.com

In the following we describe a simple optical toy model to mimic the multilayer graphene system.

First, let us consider a boundary between two regions with -for instance- different dielectric constants<sup>1</sup>. The boundary will partially reflect and partially transmit an incoming wave, from either the left or the right. See Fig. S1(a). We will take this boundary as the equivalent of a single graphene layer.

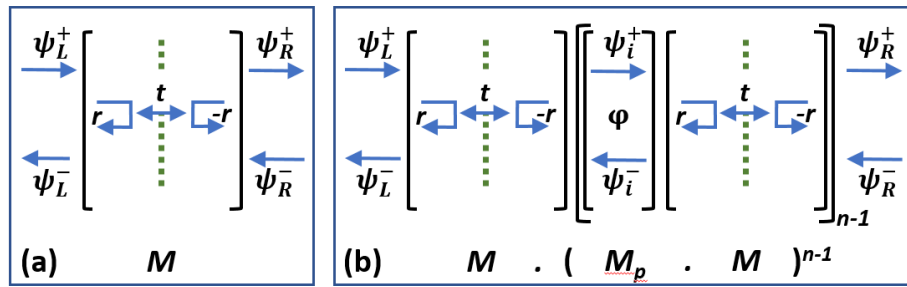

Figure S1: (a) A single boundary (green dashed line) with impinging and reflecting waves  $\psi_L^+$  and  $\psi_L^-$  to the left and  $\psi_R^+$  and  $\psi_R^-$  to the right. The boundary reflection amplitudes are given by  $r$  and  $t$ . The waves to the left and the right are coupled by the transfer matrix  $M$  (eq.(2)). (b) For a double boundary ( $n=2$ ), again we have impinging and reflecting waves  $\psi_L^+$  and  $\psi_L^-$  to the left and  $\psi_R^+$  and  $\psi_R^-$  to the right. In the internal space between the boundaries we have waves  $\psi_i^+$  and  $\psi_i^-$ . These waves gain a phase  $\varphi$  as they advance from one boundary to the next. The propagation matrix  $M_p$  from boundary to boundary is given by eq.(3), while the waves to the left and the right are coupled by the matrix product  $M.M_p.M$  (eq.(4)). For  $n$  layers, the single right-hand propagation space plus boundary is replaced by a sequence of  $(n-1)$  propagation spaces and boundaries, and the left-hand and right-hand waves are coupled by the product  $M.(M_p.M)^{n-1}$  (eq.(5)).

Assuming an incoming wave  $\psi_L^+$  approaching the boundary from the left, with reflection amplitude  $r$  and transmission amplitude  $t$ , and/or an incoming wave  $\psi_R^-$  from the right, with reflection amplitude  $-r$  and transmission amplitude  $t$ , we can write:

$$\psi_R^+ = t\psi_L^+ - r\psi_R^- \quad (1a)$$

$$\psi_L^- = r\psi_L^+ + t\psi_R^- \quad (1b)$$

The transmissivity  $T_1$  and reflectivity  $R_1$  of this single boundary are given by  $T_1 = |t|^2$  and  $R_1 = |r|^2$ . From eqs. (1) it follows that

$$\begin{pmatrix} \psi_R^+ \\ \psi_R^- \end{pmatrix} = M \begin{pmatrix} L^+ \\ L^- \end{pmatrix} = \begin{pmatrix} \frac{r^2}{t} + t & \frac{-r}{t} \\ \frac{-r}{t} & \frac{1}{t} \end{pmatrix} \begin{pmatrix} \psi_L^+ \\ \psi_L^- \end{pmatrix} \quad (2)$$

where  $M$  is the transfer matrix for the single boundary sketched in Fig. S1(a).

Instead of a single boundary we may have two boundaries, as in Fig. S1(b). We take the waves propagating from one boundary to the next to advance by a phase angle  $\varphi$  along the way ( $\psi_i^+, \psi_i^-$ ). This can be expressed by a propagation matrix  $M_p$ :

$$M_p = \begin{pmatrix} e^{i\varphi} & 0 \\ 0 & e^{-i\varphi} \end{pmatrix} \quad (3)$$

For the two-layer system it then follows that

$$\begin{pmatrix} \psi_R^+ \\ \psi_R^- \end{pmatrix} = M \cdot M_p \cdot M \begin{pmatrix} \psi_L^+ \\ \psi_L^- \end{pmatrix} \quad (4)$$

and, in general, for an  $n$ -layer system with equally spaced boundaries:

$$\begin{pmatrix} \psi_R^+ \\ \psi_R^- \end{pmatrix} = M \cdot (M_p \cdot M)^{n-1} \begin{pmatrix} \psi_L^+ \\ \psi_L^- \end{pmatrix} = \begin{pmatrix} \frac{r_n^2}{t_n} + t_n & \frac{-r_n}{t_n} \\ \frac{-r_n}{t_n} & \frac{1}{t_n} \end{pmatrix} \begin{pmatrix} \psi_L^+ \\ \psi_L^- \end{pmatrix} \quad (5)$$

Here,  $r_n$  and  $t_n$  are the reflection and transmission amplitudes of the  $n$ -layer system, in analogy with Eq. (2). The total transmissivity  $T$  and reflectivity  $R$  of the  $n$ -layer system are then  $T = |t_n|^2$  and  $R = |r_n|^2$ .

Alternatively, expressions for  $t_n$  and  $r_n$  can be obtained by the method of infinite sums<sup>2</sup>, explicitly accounting for multiple reflections and transmissions between the boundaries. For example, for Fig. S1(b) with 2 layers and a wave  $\psi_L^+$  coming in from the left:

$$t_{1,2} = t_1 e^{i\varphi} t_2 + t_1 e^{i\varphi} r_2 \cdot -r_1 e^{2i\varphi} t_2 + t_1 e^{i\varphi} r_2 \cdot -r_1 e^{2i\varphi} r_2 \cdot -r_1 e^{2i\varphi} t_2 + \dots = \frac{t_1 t_2 e^{i\varphi}}{1 + r_1 r_2 e^{2i\varphi}} \quad (6a)$$

$$r_{1,2} = r_1 + t_1 e^{2i\varphi} r_2 t_1 + t_1 e^{2i\varphi} r_2 e^{2i\varphi} \cdot -r_1 r_2 t_1 + \dots = r_1 + \frac{t_1^2 r_2 e^{2i\varphi}}{1 + r_1 r_2 e^{2i\varphi}} \quad (6b)$$

Here we have used the subscripts 1 and 2 for the 1<sup>st</sup> (left) and 2<sup>nd</sup> (right) boundary. Notice that we can go from two to three (or more) boundaries by replacing the right-hand boundary for a single layer by a composite boundary containing two (or more) layers, with  $t_2$  and  $r_2$  being the complex transmission and reflection amplitudes for this composite boundary. This leads to the following recursive relations for an  $n$ -layer system (i.e. generalized version of eqs. (6a-b)):

$$t_n = \frac{t_1 \cdot t_{n-1} e^{i\varphi}}{1 + r_1 \cdot r_{n-1} e^{2i\varphi}} \quad (7a)$$

$$r_n = r_1 + \frac{t_1^2 r_{n-1} e^{2i\varphi}}{1 + r_1 \cdot r_{n-1} e^{2i\varphi}} \quad (7b)$$

Assuming that  $t$  and  $r$  are identical for each single-layer boundary [i.e.  $t_1=t_2=t$ ,  $r_1=r_2=r$ , Fig.S1(b)], we derive explicitly for

2 layers:

$$t_2 = \frac{t^2 e^{i\varphi}}{1 + r^2 e^{2i\varphi}} \quad (8a)$$

$$r_2 = r * \frac{1 + (r^2 + t^2) e^{2i\varphi}}{1 + r^2 e^{2i\varphi}} \quad (8b)$$

3 layers:

$$t_3 = \frac{t^3 e^{3i\varphi}}{1 + 2r^2 e^{2i\varphi} + r^2 (r^2 + t^2) e^{4i\varphi}} \quad (8c)$$

$$r_3 = r * \frac{1 + (2r^2 + t^2) e^{2i\varphi} + (r^2 + t^2)^2 e^{4i\varphi}}{1 + 2r^2 e^{2i\varphi} + r^2 (r^2 + t^2) e^{4i\varphi}} \quad (8d)$$

4 layers:

$$t_4 = \frac{t^4 e^{4i\varphi}}{1 + 3r^2 e^{2i\varphi} + r^2 (3r^2 + 2t^2) e^{4i\varphi} + r^2 (r^2 + t^2)^2 e^{6i\varphi}} \quad (8e)$$

$$r_4 = r * \frac{1 + (3r^2 + t^2) e^{2i\varphi} + (3r^4 + 4r^2 t^2 + t^4) e^{4i\varphi} + (r^2 + t^2)^3 e^{6i\varphi}}{1 + 3r^2 e^{2i\varphi} + r^2 (3r^2 + 2t^2) e^{4i\varphi} + r^2 (r^2 + t^2)^2 e^{6i\varphi}} \quad (8f)$$

Obviously, with increasing numbers of layers these explicit expressions become more and more cumbersome. For numerical evaluation it is more convenient to use either eq. (5) or eqs. (7). While mathematically somewhat different, the matrix and infinite-sum approaches are of course exactly equivalent. For example, if we work out the  $1/t_n$  matrix element (lower right element, eq. (5)), we recover eq. (7a), or eqs. (8a,c,e), i.e. the repeated matrix multiplications implicitly take the infinite sums over all possible reflections/transmissions.

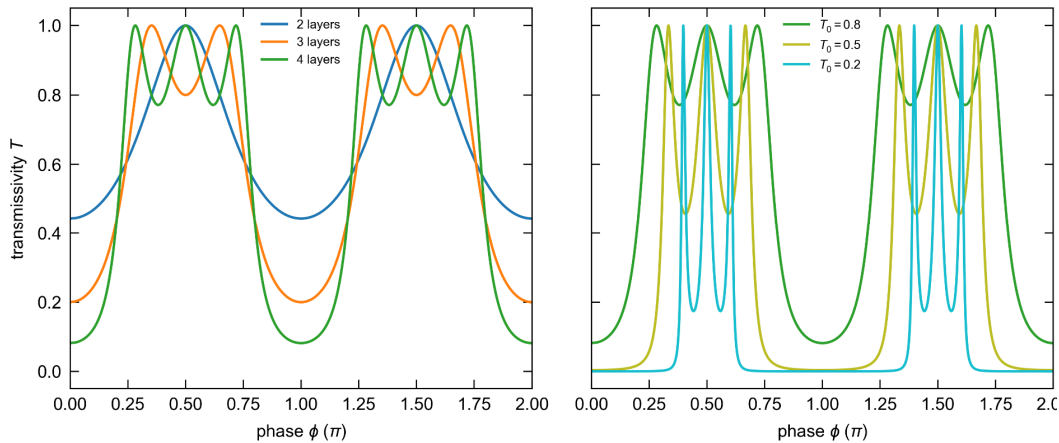

Figure S2: (a) Transmissivity  $T (=1-R)$  for 2, 3 and 4 layer systems, with single-layer  $T_1=0.8$  and  $R_1=0.2$  (no loss). For a single layer  $R$  and  $T$  are constant. The single transmission peaks at  $\varphi = \pi \left( m + \frac{1}{2} \right)$ , ( $m = 0, 1, 2, \dots$ ) for a 2-layer system split into double and triple peaks for 3- and 4-layer systems, respectively (b) Transmissivity vs  $\varphi$  for  $T_1=0.8, 0.5$ , and  $0.2$ , for 4LG. With decreasing  $T_1$  the maxima are closer together and narrower, and the minima between the peaks become deeper.

Figure S2(a) shows  $T (=1-R, \text{ i.e. no loss})$  for 1-, 2-, 3-, and 4-layer systems with single-layer  $T_1=0.8$  and  $R_1=0.2$ . The 2-layer system behaves like a perfect, optical multi-layer anti-reflection coating, with a single maximum in  $T$  (minimum in  $R$ ) at  $\varphi = \frac{\pi}{2}$ , repeating with period  $\pi$ , i.e. half wavelength spacing between boundaries. This single maximum (minimum) splits to a doublet for a 3-layer system, a triplet for a 4-layer system, etc. The magnitude of the splitting in the multilayers depends on the transmissivity of the single layer (figure S2(b)), increasing with increasing  $T_1$ . The peaks are found at

$$\varphi = \pi \left( m + \frac{1}{2} \right) \quad (2\text{LG}) \quad (9a)$$

$$\varphi = \pi m \pm \tan^{-1}(\sqrt{(4 - T_1)/T_1}) \quad (3\text{LG}) \quad (9b)$$

$$\varphi = \pi \left( m + \frac{1}{2} \right) \text{ and } \varphi = \pi m \pm \tan^{-1}(\sqrt{(2 - T_1)/T_1}) \quad (4\text{LG}) \quad (9c)$$

As  $T_1$  approaches zero, the splitting vanishes and the peak widths goes to zero, until at  $T_1=0$  the peaks have disappeared completely and the waves are fully reflected.

On the other hand, with increasing  $T_1$  the transmission window becomes broader, and the transmission oscillations between the peaks becomes shallower (figure S2(b)). Thus, the overall splitting and shape of the reflection/transmission curves contains information on the  $T_1/R_1$  ratio. For example, a relatively broad splitting with small amplitude oscillations is indicative of a large  $T_1/R_1$  ratio. We will see that this closely corresponds to the situation in graphene multilayers. In the optical system a minimum in reflectivity corresponds to destructive interference in the multiple reflections between layers, and a maximum in transmission to constructive interference in the multiple reflections between layers. The analogy with multilayer graphene suggests that the so-called ‘interlayer’ states in graphene find their origin in such constructive/destructive multi-reflection electron interferences between layers.

How far can we push this analogy? In the LEEM/eV-TEM experiments we measure  $T$  and  $R$  of the complete system of layers as a function of electron energy  $E_0$ , referenced to the vacuum level. The vacuum electron wavelength increases with the square root of electron energy. When an electron enters a graphene multilayer, it gains additional energy equal to the workfunction  $\phi_w$  (given in eV). The wavevector of the electron inside the graphene multilayer is then given by  $q = \sqrt{\frac{2m_e}{\hbar^2} (E_0 + \phi)}$ , still assuming a free-electron-like model and thus assigning to  $m_e$  the free-electron mass. (The interlayer state does in fact have an effective electron mass close to 1, so this is not unreasonable<sup>3</sup>.) When an electron advances between layers, its phase advances by  $\varphi = q \cdot d$  where  $d$  is the interlayer spacing between adjacent graphene layers. Therefore, we have a direct relation between electron energy and phase.

In general,  $R_1$  and  $T_1$  do not add up to 1. Various losses such as absorption, diffuse scattering, etc. lead to  $R_1+T_1<1$ . Also,  $R_1$  and  $T_1$  are not necessarily constant with increasing electron energy. Let us therefore assume that  $R_1$  and  $T_1$  are energy-dependent, and that losses increase with energy. Figure S3(a) shows the reflectivity  $R$  for 1- to 8-layer systems, as function of vacuum electron energy  $E_0$ , using the work function<sup>5</sup> of graphite for  $\phi$ , i.e.  $\phi = 4.6$  eV. It is assumed that for all individual layers  $R_1=0.1$  and  $T_1=0.6$  for  $E_0 < 6$  eV, decaying exponentially at higher energies, with a decay length of 9 eV, to a final value of  $R_1=0.033$  and  $T_1=0.2$ . We use the same values for Fig. 3e of the main manuscript. We compare the results predicted by this energy-dependent toy model with experimental results for multilayer graphene

on SiC(0001) obtained by Hibino et al.<sup>4</sup> [Fig. S3(b)]. The rather striking agreement between the optical model in Fig. S3(a) and the experimental data in Fig. S3(b) would suggest that this close correspondence is not accidental. Indeed, the optical model appears to capture the essential physics of the graphene multilayer. The reflectivity minima around  $\sim 3$  and  $\sim 17$  eV correspond to the 1<sup>st</sup> and 2<sup>nd</sup> anti-reflection bands in Fig. S2(a).

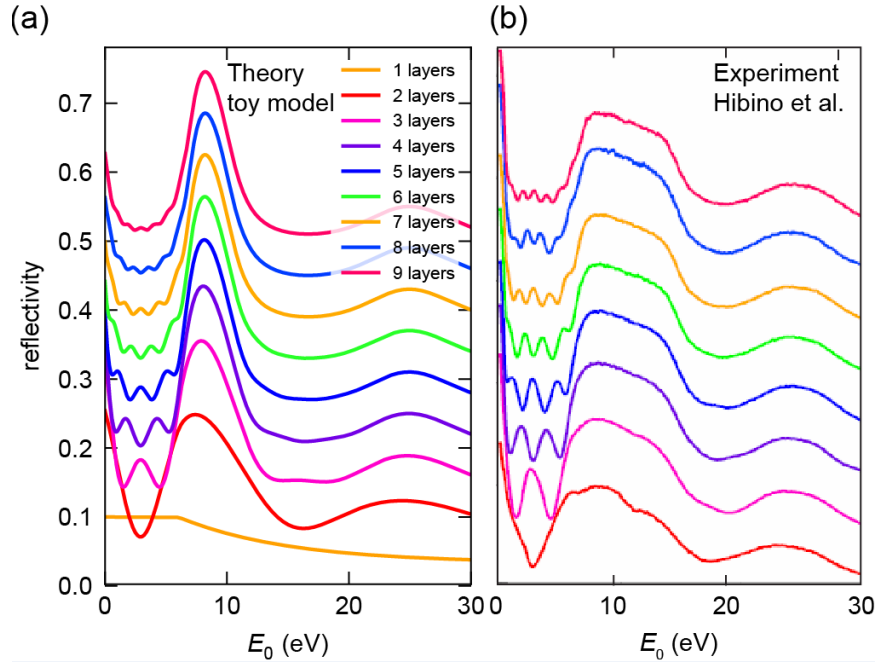

Figure S3. (a) Reflectivity for the optical toy model for 1-9 layers, with energy-dependent single-layer reflectivity as shown by the bottom, orange curve. (b) Electron specular reflectivity for 2-9 layers of graphene on SiC(0001) measured with Low Energy Electron Microscopy (adapted from ref.4).

The energy dependence of  $T_1$  and  $R_1$  was chosen to optimize agreement between Figs. S3(a) and S3(b). For example, if we choose an exponential (or linear) increase in  $T_1$  and  $R_1$  coming from 30 eV down to  $E_0=0$  eV, the lower energy oscillations are overdamped. Apparently, in the range 0-6 eV losses are rather constant. We chose a cut-off of 6 eV as the  $\pi$ -plasmon loss in graphene has an energy of  $\sim 6$  eV, so at lower electron energies this loss mechanism is inaccessible. Phonon and intra-band transitions are accessible in this low-energy range but are not strongly energy dependent. When the electron energy exceeds 6 eV,  $\pi$ -plasmon losses start to play a role, slowly increasing with energy. At  $\sim 15$  eV the  $(\sigma+\pi)$ -plasmon starts to become accessible, adding a third loss channel. So qualitatively, we expect rather fixed losses below 6 eV, and gradually increasing losses, reducing  $T_1+R_1$ , above 6 eV. With these general considerations we then optimized the energy dependence of  $T_1$  and  $R_1$  (keeping their ratio constant) to obtain the results of Fig. S3(a). We find that these same parameters also result in good agreement between optical model and experiment for the elastic and inelastic electron mean free paths discussed in the main text.

## References

1. See for instance: Dr. Hugo Anders, 'Thin Films in Optics', The Focal Press, London and New York, 1967
2. Lord Rayleigh. Proc. Roy. Soc. **93** (1917) 565
3. J. Jobst, J. Kautz, D. Geelen, R.M. Tromp, S.J. van der Molen, Nature Communications **6**, 8926 (2015).
4. H. Hibino, H. Kageshima, F. Maeda, M. Nagase, Y. Kobayashi, Y. Kobayashi, and H. Yamaguchi, E-Journal Surf. Sci. Nanotechnol. **6**, 107 (2008).
5. One may argue that instead of setting  $\phi = 4.6$  eV (the graphene workfunction) we should use the graphene inner potential, reported<sup>6-8</sup> to be between 16 and 18 eV. A value<sup>6</sup> of  $\phi = 16.4$  eV also reproduces the low energy minima in Fig. S3(a), but the energy spectrum is now significantly stretched, with the minimum around 16 eV shifting to  $\sim 25$  eV. We can fix this by using a different effective mass, and adding energy-dependent scattering phase shifts, but this would defeat the purpose of the toy model, i.e. to show the scattering resonance origin of the oscillations.
6. A. Grüneis, C. Attacalite, T. Pichler, V. Zabolotnyy, H. Shiozawa, S.L. Molodtsov, D. Inosov, A. Koitzsch, M. Knupfer, J. Schiessling, R. Follath, R. Weber, P. Rudolf, L. Wirtz, and A. Rubio, Physical Review Letters **100**, 037601 (2008).
7. S.Y. Zhou, G.-H. Gweon, and A. Lanzara, Annals of Physics **321**, 1730 (2006).
8. F. Matsui, H. Nishikawa, H. Daimon, M. Muntwiler, M. Takizawa, H. Namba, and T. Greber, Physical Review B **97**, 045430 (2018).
